# Supplementary material for: NnD: Diffusion-based Generation of Physically-Nonnegative Objects
Source: arXiv:2506.10112 ancillary file (2025-06-11)
Supplement: Supplementary file 1 [file fake_or_real_cloud.pdf]

## NnD: Diffusion-based Generation of Physically Nonnegative Objects

Authors: Nadav Torem, Yoav Schechner, Tamar Sde Chen

|       |            |
|-------|------------|
| 10083 | real cloud |
| 10106 | fake       |
| 10162 | real cloud |
| 10217 | fake       |
| 10435 | real cloud |
| 1045  | fake       |
| 10623 | fake       |
| 10740 | real cloud |
| 11100 | real cloud |
| 1131  | real cloud |
| 12060 | real cloud |
| 12116 | fake       |
| 1213  | fake       |
| 12591 | fake       |
| 12622 | real cloud |
| 13212 | real cloud |
| 13620 | real cloud |
| 1406  | fake       |
| 14940 | real cloud |
| 15089 | real cloud |
| 15109 | real cloud |

|       |            |
|-------|------------|
| 15300 | real cloud |
| 15353 | real cloud |
| 15729 | real cloud |
| 16260 | real cloud |
| 16365 | fake       |
